# Supplementary material for: Sentiment cascades in the 15M movement
Source: arXiv:1505.03776 source file (2015-05-14)
Supplement: Supplementary file 1 [file AGMS-SI.pdf]

# Sentiment cascades in the 15M movement - Supplementary Information

Raquel Alvarez and Yamir Moreno

*Institute for Biocomputation and Physics of Complex Systems,  
University of Zaragoza, Campus Rio Ebro 50018, Zaragoza, Spain*

David Garcia and Frank Schweitzer\*

*Chair of Systems Design, ETH Zurich,  
Weinbergstrasse 56/58, 8092 Zurich, Switzerland*

(Dated: April 24, 2015)

---

\*Electronic address: [dgarcia@ethz.ch](mailto:dgarcia@ethz.ch)

## I. PRESELECTED KEYWORDS

TABLE I: List of preselected keywords (hashtags) and counts of tweets.

| Keyword             | Counts | Keyword                  | Counts | Keyword           | Counts |
|---------------------|--------|--------------------------|--------|-------------------|--------|
| #acampadasol        | 189251 | #tomalaplaza             | 2684   | #dry_caceres      | 10     |
| #spanishrevolution  | 158487 | #acampadas               | 2339   | #dryasturies      | 5      |
| #nolesvotes         | 66329  | #15mpasalo               | 2336   | #democraziareale  | 4      |
| #15m                | 65962  | #cabemostodas            | 1895   | #democratiereelle | 3      |
| #nonosvamos         | 55245  | #nonosmovemos            | 1382   | #dry_cadiz        | 3      |
| #democraciarealya   | 47463  | #3puntosbasicos          | 1378   | #dry_toledo       | 3      |
| #notenemosmiedo     | 32586  | #frenchrevolution        | 1164   | #acampadasvlla    | 2      |
| #yeswecamp          | 31811  | #estonoseacaba           | 1120   | #drybizkaia       | 2      |
| #15mani             | 17986  | #acampadatoledo          | 750    | #dry_santander    | 2      |
| #acampadasevilla    | 14356  | #nonosrepresentan        | 696    | #15mayovalencia   | 1      |
| #globalcamp         | 13186  | #acampadalondres         | 627    | #dry_pisa         | 1      |
| #acampadavalencia   | 13129  | #globalrevolution        | 622    | #dryginebra       | 0      |
| #acampadagranada    | 9717   | #acampadazaragoza        | 462    | #DRY_Algeciras    | 0      |
| #acampadamalaga     | 6808   | #acampadaparis           | 438    | #demorealyaib     | 0      |
| #acampadazgz        | 6033   | #takethesquare           | 229    | #DRYGipuzkoa      | 0      |
| #consensodeminimos  | 4348   | #periodismoeticoya       | 207    | #DryValladolid    | 0      |
| #italianrevolution  | 3981   | #hastalasangenerales     | 45     | #ItalRevolution   | 0      |
| #estonosepara       | 3860   | #irishrevolution         | 39     | #BolognaDRY       | 0      |
| #acampadaalicante   | 3593   | #democraziarealeora      | 38     | #DRY_Pavia        | 0      |
| #tomalacalle        | 3517   | #democraciaparticipativa | 33     | #DRY_Almeria      | 0      |
| #europeanrevolution | 3035   | #15mpamplona             | 22     | #15mayoCordoba    | 0      |
| #acampadapamplona   | 2839   | #barcelonarealya         | 17     | #ciudades-dry     | 0      |
| #worldrevolution    | 2777   | #dry_jaen                | 12     |                   |        |
| #acampadapalma      | 2709   | #usarevolution           | 12     |                   |        |

## II. SENTIMENT ANALYSIS IN SPANISH

To extract the emotional content of tweets, we applied **SentiStrength**, a lexicon-based tool for sentiment analysis developed for English. **SentiStrength** uses a user-defined lexicon of emotional terms, negations, and booster words, allowing its application to various languages, including English, German, and Russian. It has been used in industrial applications, and can be tried online in [sentistrength.wlv.ac.uk](http://sentistrength.wlv.ac.uk). The first adaptations of **SentiStrength** to Spanish reported on its website were informally validated, which motivated us to create an independent lexicon to classify Spanish tweets. An initial version of our Spanish adaptation of **SentiStrength** was reported in a Spanish sentiment analysis workshop [1], but here we present an updated version for our study.

We started with an established lexicon of word valence in Spanish [2], in which the sentiment of 1034 words were coded based on expert ratings. We transformed the  $[1, 9]$  scale of this lexicon into the  $[-5, 5]$  scale of **SentiStrength**, and applied Kleene’s stemming to each word, having a final amount of 992 lemmas with their corresponding sentiment values. We extend this lexicon by detecting emotional terms from the TASS2013 60K dataset [3]. TASS2013 60K contains Spanish tweets preclassified as positive, negative, or neutral depending on a syndication of sentiment analysis tools and human classification. For each word contained in this corpus, we compute the log-likelihood of the word appearing in a positive and a negative tweet, and produced a rank of the most discriminative terms. After stemming, this step provided 464 stems to the lexicon, and helped us to detect two interesting emotion-bearing idioms: “buenos dias” (good morning) seems not to differentiate classes, and “lo siento” (I’m sorry) is very discriminative for the negative class in comparison to the term “siento”(feel). This also allowed us to fine-tune the table of emoticons of **SentiStrength**, as one emoticon of 2 to 3 characters within a tweet of 140 carries a lot of emotional content.

We manually translated the lists of booster terms and negations of the current version of **SentiStrength** for English into Spanish. Due to the short length of tweets, we chose to leave out the spell checking option of **SentiStrength** and the rule of boosting by using repeated letters. These rules require additional lexica of word normalization, which are yet to be developed and tested for Spanish. In our classification, only explicit diminishing terms reduce the evidence of sentiment in a Tweet. Before classifying tweets, we collapse diacritic

accents to their ASCII version, to ensure the correct execution of **SentiStrength**.

We validate this unsupervised classification in 3 ways:

1. We compare with the sentiment in the TASS2013 60K dataset, comparing our results with its semiautomatically classified sentiment values.
2. We evaluate our classification against the TASS2013 7K dataset, which is of smaller size but contains sentiment classes manually annotated without the support of any sentiment analysis tool. This dataset is disjoint to the previous one, and serves as a test leave-out sample for our adaptation of **SentiStrength**.
3. From the previous two datasets, manual tags of tweet topics are available. We use these tags to extract two subdatasets of tweets related to political and economical topics. These two sets of tweets will allow us to understand better how our classification tool performs for tweets similar to the topics of 15M, which are mainly social, political, and economical. Note that these two datasets are a subset of the two previous ones, and that they are not disjoint.

TABLE II: **Classification results for the TASS datasets**

|          | 60K dataset |       |       |       | 7K dataset |       |       |       |
|----------|-------------|-------|-------|-------|------------|-------|-------|-------|
| class    | $B_c$       | $P_c$ | $R_c$ | $F_c$ | $B_c$      | $P_c$ | $R_c$ | $F_c$ |
| positive | 0.366       | 0.613 | 0.794 | 0.692 | 0.399      | 0.632 | 0.783 | 0.699 |
| negative | 0.26        | 0.612 | 0.675 | 0.642 | 0.302      | 0.68  | 0.635 | 0.657 |
| neutral  | 0.374       | 0.682 | 0.436 | 0.532 | 0.298      | 0.569 | 0.424 | 0.486 |
| accuracy | 0.629       |       |       |       | 0.631      |       |       |       |

The results of the first two evaluation steps are reported in Table II, achieving an overall accuracy above 60% for both datasets, and with precision and recall values significantly larger than the base rates of each class. The result of the evaluation of topics is shown in Table III, showing that accuracy is similar for economics as for the above results. The quality of the classification decreases slightly for the classification of tweets related to politics, in line with previous results [4]. A possible explanation for this effect is the common presence of sarcasm when discussing political topics, which difficulties the classification task. Nevertheless,

TABLE III: **Classification results for the topics of politics and economics**

|          | politics |       |       |       | economics |       |       |       |
|----------|----------|-------|-------|-------|-----------|-------|-------|-------|
| class    | $B_c$    | $P_c$ | $R_c$ | $F_c$ | $B_c$     | $P_c$ | $R_c$ | $F_c$ |
| positive | 0.146    | 0.383 | 0.589 | 0.464 | 0.256     | 0.482 | 0.705 | 0.572 |
| negative | 0.65     | 0.788 | 0.794 | 0.791 | 0.385     | 0.673 | 0.678 | 0.675 |
| neutral  | 0.204    | 0.417 | 0.248 | 0.311 | 0.359     | 0.615 | 0.406 | 0.489 |
| accuracy | 0.587    |       |       |       | 0.652     |       |       |       |

accuracy values are comparable to the results of the 7K dataset, allowing the application of this adaptation of **SentiStrength** to the emotions expressed in the tweets of the 15M movement.

We compute the overall ratios of positive, negative, and neutral tweets over three different datasets: (i) a random sample of more than 144 Million tweets in Spanish from the **Twitter** gardenhose, (ii) the set of tweets related to the 15M movement, and (iii) the sample of individual tweets from the timelines of the users involved in the movement. The ratios of positive, negative, and neutral tweets are very similar for both the 15M tweets and the samples from user timelines. This verifies that the tweets about the movement are broad enough to show an emotionality similar to any other tweet of the daily experience of the participants. The random sample, however, shows a different pattern, where the ratio of positive tweets is higher and the ratios of neutral and negative tweets are lower. This can be attributed to the mixed nature of **Twitter**, as it does not only serve as a social medium, but also as a news and marketing site [5]. This stronger positive bias can be due to advertisement and retweets, as well as due to dialectal variations of Spanish from places other than Spain. Due to this difference between random tweets and tweets from Spanish users, we chose to standardize our metrics based on the users of the 15M dataset, and not over the larger, but less representative, random sample from the gardenhose.

TABLE IV: Emotional expression counts and ratios

| Dataset     | Size (Tweets) | Positive           | Neutral            | Negative           |
|-------------|---------------|--------------------|--------------------|--------------------|
| random      | 144,814,110   | 74,606,540 (51.5%) | 38,790,342 (26.8%) | 31,417,227 (21.7%) |
| 15M         | 556,334       | 256,964 (46.2%)    | 175,336 (31.5%)    | 124,034 (22.3%)    |
| individuals | 15,411,025    | 7,201,200 (46.7%)  | 4,782,556 (31.0%)  | 3,427,269 (22.2%)  |

### III. EMOTION CASCADE SIZE DISTRIBUTION ANALYSIS

Kolmogorov-Smirnov tests validate the observation that both spreader and information cascades are different when they carry both negative and positive emotional content, i.e. when the expression of sentiment in their tweets is polarized. We applied a correction factor to the KS statistic of cascade size distributions, explained in [6]. This factor allows us to reject the null hypothesis that positive activity and information cascades have the same size as their neutral and negative counterparts.

To further compare these cascades, we fitted power law distributions of the form  $p(x) \sim x^{-\alpha}$  for  $x \geq x_{min}$ , to the empirical distributions of  $n_{sp}$  and  $n_c$ . To do so, we made use of the Python module *powerlaw* [7]. We also investigated the goodness of the fits by comparing them to fits to other distributions. In this way we are able to identify if a power law behavior is a good description of our data. Specifically, we show the likelihood ratio,  $R$ , between the power law and a log-normal distribution, and the corresponding  $p$ -value indicating the significance for the observed likelihood direction. Positive values of  $R$  suggest that the data is more likely drawn from a power law distribution. However, when these values are obtained in combination with high  $p$ -values ( $p > 0.05$ ), the evidence of a power law behavior is moderated.

### IV. INITIAL TWEET EMOTIONS ANALYSIS

Is the larger size of negative and neutral cascades due to the collective emotions of the participants, or does it uniquely depend on the spreading power of the emotions in the tweet that triggered the cascade?

To answer this question, we divide cascades according to the sentiment in their initial

|            | Activity cascades |         | Information cascades |         |
|------------|-------------------|---------|----------------------|---------|
| Test       | KS                | p-value | KS                   | p-value |
| Pos vs Neg | 0.026             | 0.000   | 0.032                | 0.000   |
| Pos vs Neu | 0.111             | 0.000   | 0.024                | 0.000   |
| Neg vs Neu | 0.143             | 0.000   | 0.009                | 0.285   |
| Pos vs Bip | 0.926             | 0.000   | 0.597                | 0.000   |
| Neg vs Bip | 0.933             | 0.000   | 0.575                | 0.000   |
| Neu vs Bip | 0.897             | 0.000   | 0.581                | 0.000   |

TABLE V: KS test for CCDF of amount of spreaders and listeners depending on the aggregate sentiment.

TABLE VI: **Power law fit results for  $n_{sp}$  and  $n_c$  depending on emotion class of the cascade.**

|          | Activity cascades $n_{sp}$ |                 |           |       |             | Information cascades $n_c$ |                 |           |       |             |
|----------|----------------------------|-----------------|-----------|-------|-------------|----------------------------|-----------------|-----------|-------|-------------|
| class    | $\alpha$                   | $\sigma_\alpha$ | $x_{min}$ | KS    | R           | $\alpha$                   | $\sigma_\alpha$ | $x_{min}$ | KS    | R           |
| Positive | 2.44                       | 0.07            | 4         | 0.039 | +1.00(0.31) | 2.01                       | 0.02            | 51        | 0.009 | -0.94(0.34) |
| Negative | 1.92                       | 0.07            | 7         | 0.032 | +1.00(0.32) | 1.80                       | 0.01            | 9         | 0.012 | +1.73(0.08) |
| Neutral  | 1.95                       | 0.09            | 14        | 0.081 | +0.63(0.53) | 1.84                       | 0.01            | 18        | 0.007 | +0.79(0.43) |
| Bipolar  | 2.74                       | 0.32            | 8         | 0.086 | +0.77(0.32) | 1.99                       | 0.08            | 157       | 0.043 | -0.42(0.67) |

tweets  $e_i$ , which is 1, 0, or  $-1$ , and compute the sizes of information and activity cascades for each type of initial tweet. Cascade size distributions for each kind of initial tweet are displayed in Figure 1 and disclosed in Tables VII and VIII in the SI. Two-sample Kolmogorov-Smirnov tests of information cascade sizes gave  $p$ -values  $\leq 0.001$  and distance estimates below 0.05, showing that the distributions of information cascade sizes are significantly different for different sentiments in the first tweet, but the distance between distributions is too small to conclude that there is a practical effect. This way, we cannot conclude that the three distributions of information cascade sizes are the same, but that their difference is very small.

The exponents of power-law fits are barely differ between the cascade size distributions

FIG. 1: Complementary cumulative density function (CCDF) of the size of activity cascades (left), and of information cascades (right). Cascades have been divided into three groups, according to the sentiment of the initial tweet.

| Test                     | Activity cascades |         | Information cascades |        |
|--------------------------|-------------------|---------|----------------------|--------|
|                          | KS                | p-value | KS                   | pvalue |
| $e_i = -1$ vs $e_i = 0$  | 0.002             | 0.615   | 0.029                | 0.000  |
| $e_i = -1$ vs $e_i = +1$ | 0.007             | 0.000   | 0.043                | 0.000  |
| $e_i = 0$ vs $e_i = +1$  | 0.005             | 0.001   | 0.013                | 0.000  |

TABLE VII: KS test results for CCDF of distributions of  $n_{sp}$  and  $n_c$  depending on the sentiment of the initial tweet  $e_i$ .

of different  $e_i$ , having values around  $\alpha = 1.89$ . This indicates that information cascade sizes have similar scaling properties regardless of the emotion in their initial tweet, and that cascade sizes are linked to collective emotions and not to the content of a singular tweet. The same conclusion seems to hold for activity cascades. The exponents of power-law fits reveal that activity cascades triggered by positive and neutral tweets are similar, having values around  $\alpha = 2.2$ . The only notable difference is for negative tweets, suggesting that more people participate if the initial sentiment is negative, although the exponent,  $\alpha = 1.94 \pm 0.04$ , is too close to 2 to reach a conclusion about its scaling properties.

TABLE VIII: Power law fit results for  $n_{sp}$  and  $n_c$  depending on  $e_i$ .

|       | Activity cascades $n_{sp}$ |                 |           |      |             | Information cascades $n_c$ |                 |           |       |               |
|-------|----------------------------|-----------------|-----------|------|-------------|----------------------------|-----------------|-----------|-------|---------------|
| $e_i$ | $\alpha$                   | $\sigma_\alpha$ | $x_{min}$ | KS   | R           | $\alpha$                   | $\sigma_\alpha$ | $x_{min}$ | KS    | R             |
| +1    | 2.22                       | 0.03            | 7         | 0.02 | +1.00(0.32) | 1.895                      | 0.003           | 8         | 0.005 | +3.036(0.002) |
| 0     | 2.19                       | 0.02            | 5         | 0.04 | +3.32(0.00) | 1.864                      | 0.005           | 24        | 0.005 | +0.003(0.998) |
| -1    | 1.94                       | 0.04            | 12        | 0.03 | +2.25(0.02) | 1.921                      | 0.007           | 38        | 0.012 | +4.077(0.000) |

## V. SOCIAL AND COGNITIVE CASCADE DISTRIBUTION ANALYSIS

|                       | Activity cascades |         | Information cascades |         |
|-----------------------|-------------------|---------|----------------------|---------|
| Test                  | KS                | p-value | KS                   | p-value |
| High vs Low Cognitive | 0.077             | 0.000   | 0.006                | 0.427   |
| High vs Low Social    | 0.195             | 0.000   | 0.056                | 0.000   |

TABLE IX: KS test for CCDF of amount of spreaders and listeners depending on the aggregate psycholinguistic class.

TABLE X: Power law fit results for  $n_{sp}$  and  $n_c$  depending on social and cognitive content of the cascade.

|                | Activity cascades $n_{sp}$ |                 |           |      |             | Information cascades $n_c$ |                 |           |       |             |
|----------------|----------------------------|-----------------|-----------|------|-------------|----------------------------|-----------------|-----------|-------|-------------|
| ling. content  | $\alpha$                   | $\sigma_\alpha$ | $x_{min}$ | KS   | R           | $\alpha$                   | $\sigma_\alpha$ | $x_{min}$ | KS    | R           |
| High social    | 1.87                       | 0.09            | 13        | 0.03 | +1.00(0.32) | 1.66                       | 0.01            | 11        | 0.011 | +0.99(0.32) |
| Low social     | 2.33                       | 0.07            | 6         | 0.02 | +0.29(0.77) | 1.98                       | 0.02            | 56        | 0.007 | -0.73(0.47) |
| High cognitive | 2.08                       | 0.07            | 6         | 0.02 | +1.00(0.32) | 1.87                       | 0.01            | 22        | 0.007 | +0.57(0.57) |
| Low cognitive  | 2.24                       | 0.07            | 6         | 0.04 | +1.07(0.28) | 1.92                       | 0.01            | 39        | 0.006 | +1.18(0.24) |

## VI. INDIVIDUAL REGRESSION RESULTS

|                | $n(u)$    | $k_c(u)$  | $k_{in}(u)$ | $k_{out}(u)$ | $pos(u)$  | $neg(u)$  | $soc(u)$  | $cog(u)$  |
|----------------|-----------|-----------|-------------|--------------|-----------|-----------|-----------|-----------|
| $n(u)$         |           | 0.094***  | 0.007**     | 0.029***     | 0.008*    | 0.021***  | -0.023*** | -0.005    |
| $k_c(u)$       | 0.193***  |           | 0.684***    | 0.170***     | 0.008     | 0.021***  | -0.026*** | -0.006    |
| $k_{in}(u)$    | 0.015**   | 0.676***  |             | 0.204***     | -0.008    | -0.013**  | 0.012*    | -0.009    |
| $k_{out}(u)$   | 0.032***  | 0.090***  | 0.110***    |              | 0.000     | -0.001    | -0.004    | 0.000     |
| $pos(u)$       | 0.010*    | 0.005     | -0.005      | 0.000        |           | -0.457*** | 0.047***  | 0.113***  |
| $neg(u)$       | 0.026***  | 0.012***  | -0.008**    | -0.001       | -0.458*** |           | -0.030*** | 0.122***  |
| $soc(u)$       | -0.022*** | -0.012*** | 0.006*      | -0.004       | 0.037***  | -0.024*** |           | -0.094*** |
| $cog(u)$       | -0.005    | -0.003    | -0.004      | 0.000        | 0.091***  | 0.098***  | -0.095*** |           |
| Intercept      | 0.000     | 0.000     | 0.000       | 0.000        | 0.000     | 0.000     | 0.000     | 0.000     |
| R <sup>2</sup> | 0.048     | 0.537     | 0.531       | 0.126        | 0.214     | 0.217     | 0.014     | 0.024     |

TABLE XI: Linear regression results for individual activity level and network position. \*\*\* $p < 0.001$ , \*\* $p < 0.01$ , \* $p < 0.05$

- 
- [1] Garcia, D. & Thelwall, M. Political alignment and emotional expression in spanish tweets. In *Workshop on Sentiment Analysis at SEPLN*, 151– 159 (2013).
- [2] Redondo, J., Fraga, I., Padrn, I. & Comesaa, M. The spanish adaptation of anew (affective norms for english words). *Behavior Research Methods* **39**, 600–605 (2007).
- [3] Daz Esteban, A., Alegra, I. & Villena Romn, J. *Proceedings of the TASS workshop at SEPLN 2013. Actas del XXIX Congreso de la Sociedad Espaola de Procesamiento de Lenguaje Natural. IV Congreso Espaol de Informtica* (SEPLN, 2013). URL <http://www.congresocedi.es/images/site/actas/ActasSEPLN.pdf>.
- [4] Thelwall, M. *et al.* Damping sentiment analysis in online communication: Discussions, monologs and dialogs. In *Computational Linguistics and Intelligent Text Processing(Lecture Notes in Computer Science)*, vol. 7817, 1–12 (2013).
- [5] Kwak, H., Lee, C., Park, H. & Moon, S. What is twitter, a social network or a news media? In *Proceedings of the 19th International Conference on World Wide Web, WWW '10*, 591–600 (2010).
- [6] Clauset, A., Shalizi, C. R. & Newman, M. E. Power-law distributions in empirical data. *SIAM review* **51**, 661–703 (2009).
- [7] Alstott, J., Bullmore, E. & Plenz, D. powerlaw: A python package for analysis of heavy-tailed distributions. *PLoS ONE* **9**, e95816 (2014).
